# Supplementary material for: Reevaluating Convolutional Neural Networks for Spectral Analysis: A Focus on Raman Spectroscopy
Source: arXiv:2509.25964 source file (2025-09-30)
Supplement: Supplementary file 1 [file Soysal_Supporting_Information.pdf]

# Supporting Information:

## Reevaluating Convolutional Neural Networks for Spectral Analysis: A Focus on Raman Spectroscopy

Deniz Soysal,<sup>†</sup> Xabier García–Andrade,<sup>†</sup> Laura E. Rodriguez,<sup>‡</sup> Pablo Sobron,<sup>¶</sup>  
Laura M. Barge,<sup>§</sup> and Renaud Detry<sup>\*,||,⊥</sup>

<sup>†</sup>*KU Leuven, Kasteelpark Arenberg 10, 3001 Leuven, Belgium*

<sup>‡</sup>*Lunar & Planetary Institute, Universities Space Research Association, 3600 Bay Area  
Boulevard, Houston, TX 77058, USA*

<sup>¶</sup>*Impossible Sensing, 20 South Sarah Street, St. Louis, MO 63108, USA*

<sup>§</sup>*Jet Propulsion Laboratory, California Institute of Technology, 4800 Oak Grove Drive, La  
Cañada Flintridge, CA 91011, USA*

<sup>||</sup>*KU Leuven, Dept. Electrical Engineering, Research Unit Processing Speech and Images  
(PSI), Kasteelpark Arenberg 10, 3001 Leuven, Belgium*

<sup>⊥</sup>*KU Leuven, Dept. Mechanical Engineering, Research Unit Robotics, Automation and  
Mechatronics (RAM), Celestijnenlaan 300, 3001 Leuven, Belgium*

E-mail: renaud.detry@kuleuven.be

This Supporting Information provides a high-level overview of Raman spectroscopy and machine learning methodologies, aiming to bridge the knowledge gap between spectroscopy experts and machine learning practitioners. It consists of 29 pages and 20 figures.

# Raman Spectroscopy

Raman spectroscopy relies on the principle of **inelastic scattering**<sup>1</sup> of photons by a material. This scattering process is governed by the vibrational modes of molecules, which depend on both chemical bonding and structural symmetry. Consequently, a Raman spectrum serves as a **molecular fingerprint**, enabling the identification and structural analysis of chemical compounds.

Figure S1 illustrates the typical workflow of Raman spectroscopy. A laser illuminates the sample, causing the molecules to scatter light. The frequency shift between the incident and scattered photons corresponds to molecular vibrations and encodes information about the sample’s chemical structure. The scattered light is collected by a lens and directed through a monochromator to produce a spectrum.

The resulting raw spectrum plots signal intensity as a function of Raman shift (in  $\text{cm}^{-1}$ ). To enhance interpretability, this signal is typically preprocessed. Standard preprocessing steps include baseline correction, spectral truncation to focus on informative regions, and normalization. From the processed spectrum, scientists identify peak positions and intensities to determine the molecular composition of the sample.

## Data-Driven Signal Interpretation

Machine learning (ML) provides effective tools for interpreting complex signals, including Raman spectra. A central goal in ML is to learn a function that maps inputs to outputs using a dataset of observed examples. In this context, the input is typically a Raman spectrum, and the output is a corresponding mineral class.

Formally, a classification dataset consists of  $M$  samples  $\{(x_i, y_i)\}_{i=1}^M$ , where  $x_i \in \mathcal{X}$  represents an input instance (e.g., a spectrum), and  $y_i \in \mathcal{Y}$  is the associated label. The input space

---

<sup>1</sup>In inelastic scattering, the incident photon interacts with a molecule, resulting in a gain or loss of energy. In contrast, elastic scattering conserves energy. Raman spectroscopy exploits inelastic scattering to probe molecular vibrations.

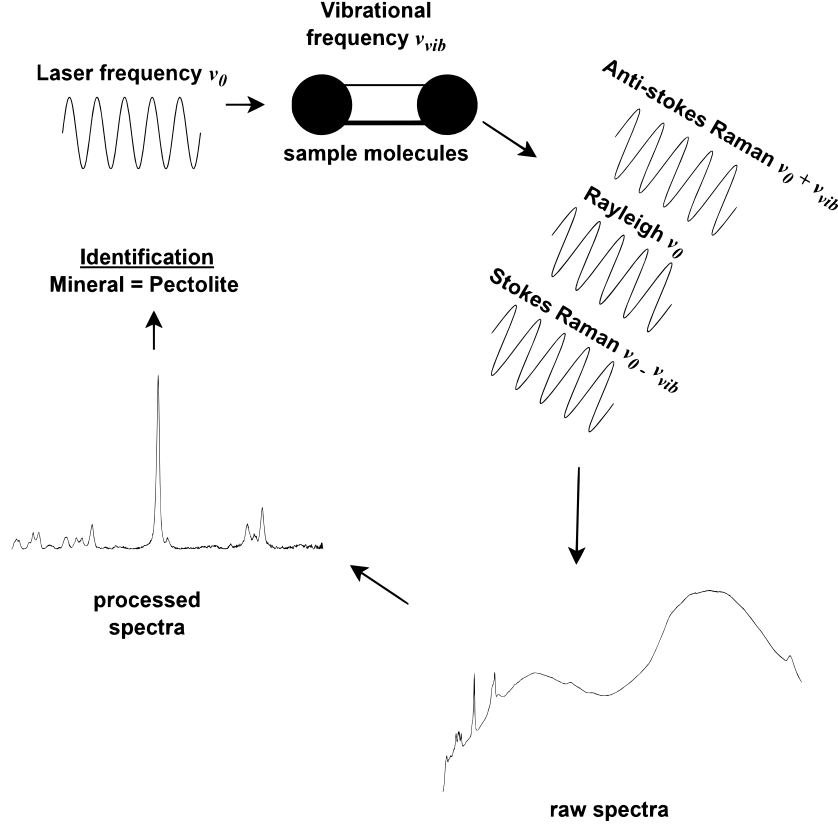

Figure S1: Schematic representation of Raman spectroscopy for mineral identification. A monochromatic laser source excites molecular vibrations within the sample, resulting in inelastic scattering. The spectrum consists of Rayleigh (elastic), Stokes, and anti-Stokes (inelastic) components, depending on the vibrational frequency  $\nu_{\text{vib}}$ . The raw spectrum is then preprocessed to remove baseline drift and enhance resolution, enabling accurate identification of the mineral species—in this case, Pectolite.

$\mathcal{X}$  is often multidimensional. In Raman spectroscopy,  $x_i$  is usually a vector in  $\mathbb{R}^S$ , where  $S$  denotes the number of sampled Raman shift positions. Additional contextual features, such as the laser excitation wavelength, can be included, in which case  $x_i \in \mathbb{R}^S \times \mathbb{R}^+$ .

The label space  $\mathcal{Y}$  consists of discrete values representing the possible classes, so that  $y_i \in \{1, 2, \dots, N\}$ , where  $N$  is the number of mineral types. The goal is to approximate a mapping function  $f_\theta : \mathcal{X} \rightarrow \mathcal{Y}$ , parameterized by  $\theta$ , that predicts the correct label  $y_i$  given an input  $x_i$ .

To train this model, a loss function  $L(y_i, f(x_i))$  quantifies the error between the predicted and actual labels. A widely used loss for multi-class classification is the categorical cross-

entropy:

$$L(y_i, f(x_i)) = - \sum_{k=1}^N y_{ik} \log \hat{y}_{ik}, \quad (1)$$

where  $\hat{y}_{ik} = f(x_i)$  is the predicted probability of class  $k$ , and  $y_{ik}$  is a one-hot encoded ground truth label. The model is trained by minimizing the total loss over the dataset:

$$\theta^* = \arg \min_{\theta} \sum_{i=1}^M L(y_i, f_{\theta}(x_i)). \quad (2)$$

The discussion thus far assumes a supervised learning setting, where each spectrum  $x_i$  has an associated ground-truth label  $y_i$ . In contrast, unsupervised learning methods operate on unlabeled data and aim to uncover structure within the input space—for instance, clustering spectra that likely belong to the same mineral class. Techniques such as  $k$ -means clustering,<sup>S1</sup> principal component analysis (PCA),<sup>S2,S3</sup> and generative modeling<sup>S4</sup> are commonly applied.

Adopting ML for spectral classification arises from the intrinsic difficulty of writing explicit rules to differentiate mineral classes based solely on Raman features. Spectral variability, peak overlaps, and noise make manual rule-based approaches impractical. In contrast, ML models trained on labeled examples can automatically learn discriminative patterns in the data, without requiring hand-crafted rules or domain-specific heuristics.

Having introduced the fundamental concepts and terminology, the remainder of this section focuses on several representative ML methods applied in the classification of Raman spectra: Support Vector Machines (SVMs),  $k$ -Nearest Neighbors (KNN), and deep learning techniques such as Convolutional Neural Networks (CNNs).

## Support Vector Machines (SVM)

Support Vector Machines (SVMs), introduced by Vapnik *et al.*,<sup>S5</sup> are methods used for classification and function estimation tasks. Their core principle is *margin maximization*: identifying a hyperplane that separates data from different classes with the largest possible

margin. This margin corresponds to the distance between the hyperplane and the closest samples from each class, known as *support vectors*. These critical data points determine the orientation and position of the decision boundary.

**Linear Case** Consider a binary classification dataset  $\{(x_k, y_k)\}_{k=1}^N$ , where  $x_k \in \mathbb{R}^S$  are input features and  $y_k \in \{-1, +1\}$  are class labels. A linear SVM seeks a weight vector  $W$  and bias  $b$  such that the decision function

$$\hat{y} = \text{sign}(W^\top x + b) \quad (3)$$

correctly classifies the training data. To ensure correct classification, the model must satisfy:

$$\begin{aligned} W^\top x_k + b &\geq 1 & \text{if } y_k = +1, \\ W^\top x_k + b &\leq -1 & \text{if } y_k = -1. \end{aligned} \quad (4)$$

These constraints can be unified as:

$$y_k(W^\top x_k + b) \geq 1 \quad \forall k. \quad (5)$$

The optimal hyperplane is obtained by solving the following convex optimization problem:

$$\begin{aligned} \min_{W, b} \quad & \frac{1}{2} \|W\|^2 \\ \text{subject to} \quad & y_k(W^\top x_k + b) \geq 1, \quad \forall k. \end{aligned} \quad (6)$$

This formulation maximizes the margin  $2/\|W\|$  between the two classes. However, real-world data often contain noise or overlapping classes, which make the data not perfectly separable. To accommodate misclassifications, slack variables  $\xi_k \geq 0$  are introduced, yielding the soft-margin SVM:

$$\min_{W, b, \xi} \quad \frac{1}{2} \|W\|^2 + C \sum_{k=1}^N \xi_k \quad (7)$$

$$\text{subject to} \quad y_k(W^\top x_k + b) \geq 1 - \xi_k, \quad \xi_k \geq 0,$$

where  $C > 0$  is a regularization parameter controlling the trade-off between maximizing the margin and minimizing classification errors.

**Nonlinear Case** When the data are not linearly separable, SVMs can still be applied by transforming the input into a higher-dimensional space using a mapping  $\Phi(x)$ . In this transformed space, a linear hyperplane may be sufficient for separation:

$$\hat{y} = \text{sign}(W^\top \Phi(x) + b). \quad (8)$$

Direct computation in high-dimensional feature spaces can be computationally expensive. To address this, the *kernel trick* is used: inner products  $\Phi(x)^\top \Phi(y)$  are replaced by a kernel function  $K(x, y)$ , allowing the SVM to operate implicitly in the high-dimensional space:

$$K(x, y) = \Phi(x)^\top \Phi(y). \quad (9)$$

Popular kernel functions include the polynomial kernel, the radial basis function (RBF) kernel, and the sigmoid kernel. The choice of kernel significantly impacts the model's expressiveness and generalization.

**Key Hyperparameters** The performance of an SVM depends on proper tuning of the following hyperparameters:

- **Kernel function**  $K(x, y)$ : Defines the nature of the non-linear transformation applied to the data. The choice of kernel affects the flexibility of the decision boundary
- **Regularization parameter**  $C$ : Balances margin maximization with classification error. A smaller  $C$  allows for a wider margin but may increase misclassifications (un-

derfitting), while a larger  $C$  aims to classify all training examples correctly but may lead to a smaller margin and overfitting.

- **Kernel coefficient  $\gamma$ :** Defines the distance of influence of a data point. For a radial basis function kernel, it is inversely proportional to the variance of the Gaussian distribution. For low values of  $\gamma$ , further data points are considered as belonging to the same class. For high values of  $\gamma$ , the data points need to be closer to be considered as belonging to the same class.

**Practical Considerations** Several practical aspects must be addressed when applying SVMs:

- **Feature scaling** is essential to prevent features with larger magnitudes from dominating the optimization. Standardization or normalization is recommended.
- **Computational cost** can be significant for large datasets, as SVMs solve a quadratic programming problem. Efficient solvers and approximations may be needed for scalability.
- **Memory usage** can be high, especially when many support vectors are retained. This also affects prediction speed.
- **Model selection** requires careful cross-validation to choose appropriate values for  $C$ ,  $\gamma$ , and the kernel type.
- **Class imbalance** can bias the model toward majority classes. Techniques such as class weighting or resampling are often necessary.
- **Outlier sensitivity** can degrade performance, as outliers may become support vectors. Preprocessing to detect and remove such points improves robustness.

## k-Nearest Neighbors (KNN)

The  $k$ -nearest neighbors (KNN) algorithm, introduced by Cover *et al.*,<sup>S6</sup> is a non-parametric method used for classification and regression. In classification tasks, KNN assigns a label to an unlabeled data point  $\hat{x}$  based on the majority class among its  $k$  closest neighbors in the training set. Unlike model-based methods such as SVM, KNN is an instance-based approach. It does not build an explicit model during training but instead retains the entire dataset and performs classification at inference time.

To classify a new point  $\hat{x}$ , the algorithm computes its distance to each sample  $x_i$  in the training set  $X = \{x_1, x_2, \dots, x_M\}$  using a specified distance metric  $D(x_i, \hat{x})$ . Common choices include the Euclidean, Manhattan, and Mahalanobis distances. After ranking the distances, the  $k$  closest samples are selected, and the most frequent class among them is assigned to  $\hat{x}$ .

**Key Parameters** Two primary parameters influence KNN performance:

- **Distance metric:** Determines how similarity is measured between samples. The choice of metric affects how neighborhoods are formed in the feature space.
- **Number of neighbors  $k$ :** Controls the smoothness of the decision boundary. A small  $k$  (e.g.,  $k = 1$ ) makes the algorithm highly sensitive to noise (overfitting), while a larger  $k$  smooths out decision boundaries but may reduce sensitivity to local patterns (underfitting).

**Practical Considerations** Several factors should be considered when applying KNN in practice:

- **Feature scaling** is essential, as KNN relies on distance computations. Unscaled features can disproportionately influence results. Standardization or normalization is typically required.



- **Prediction cost** is high because the algorithm must compute distances to all training points at inference time. Efficient data structures (e.g., KD-trees or ball trees) can partially mitigate this cost.
- **Memory usage** grows linearly with dataset size since all training data must be stored. This can become a limiting factor for large datasets.
- **Curse of dimensionality** affects KNN performance in high-dimensional spaces, where distances lose discriminative power. Dimensionality reduction (e.g., PCA) is often necessary.
- **Sensitivity to noise and irrelevant features** can degrade classification accuracy. Feature selection or extraction helps improve robustness.
- **Class imbalance** may cause KNN to favor the majority class. Weighting neighbors inversely by distance or adjusting class priors can mitigate this issue.
- **Model selection** involves choosing the optimal value of  $k$  via cross-validation, similar to hyperparameter tuning in SVMs.

## Deep Learning

After discussing traditional machine learning approaches such as Support Vector Machines and  $k$ -Nearest Neighbors, we now turn to deep learning, with a particular focus on neural networks.

While conventional algorithms can be effective for certain tasks, they often rely on hand-crafted features and may struggle to capture the complex, high-dimensional patterns inherent in Raman spectra. These spectra frequently exhibit overlapping, subtle, and nonlinear features resulting from diverse molecular vibrations. Deep learning models, particularly neural networks with multiple layers, have demonstrated strong capabilities in modeling such complexity. By learning hierarchical representations directly from raw data, these models can

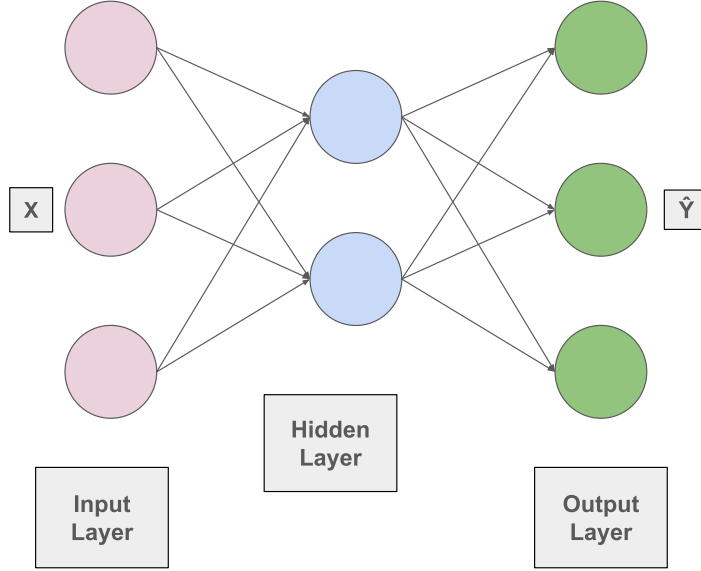

Figure S2: Schematic representation of a multilayer perceptron (MLP).

automatically extract discriminative features, making them especially suitable for Raman spectral classification.

Deep learning is founded on artificial neural networks—computational architectures inspired by biological neural systems. A neural network learns to model relationships between inputs and outputs by adjusting its internal parameters during training.

Neural networks consist of layers of interconnected computational units called *neurons*, as shown in Figure S2. These layers include an input layer, one or more hidden layers, and an output layer. In this discussion, we focus on the multilayer perceptron (MLP) with a single hidden layer, although deeper networks are commonly used in practice.

Each neuron is associated with two parameters: weights ( $\theta$ ) and a bias term ( $b$ ). When an input vector  $X$  is fed into the network, each neuron performs a linear transformation:

$$Z = \theta \cdot X + b, \quad (10)$$

followed by a non-linear activation function  $g(\cdot)$  to introduce non-linearity into the model:

$$A = g(Z) = g(\theta \cdot X + b), \quad (11)$$

where  $A$  denotes the neuron's activation. These computations are applied layer by layer in what is known as the *feedforward* step, culminating in a network output  $\hat{y}$ .

Learning occurs during the *backward* step through a process called *backpropagation*, which uses the chain rule to compute the gradients of the loss function with respect to each parameter in the network. These gradients are then used to update the parameters via gradient descent. For instance, the partial derivatives required during backpropagation are given by:

$$\frac{\partial L}{\partial \theta^{[L]}} = \frac{1}{N} \frac{\partial L}{\partial Z^{[L]}} A^{[L-1]\top}, \quad (12)$$

$$\frac{\partial L}{\partial b^{[L]}} = \frac{1}{N} \sum_{i=1}^N \frac{\partial L}{\partial Z^{[L](i)}}, \quad (13)$$

$$\frac{\partial L}{\partial A^{[L-1]}} = (\theta^{[L]})^\top \frac{\partial L}{\partial Z^{[L]}}, \quad (14)$$

where  $L$  is the loss function,  $\theta^{[L]}$  the weights in layer  $L$ ,  $Z^{[L]}$  the pre-activation output,  $A^{[L-1]}$  the activation from the previous layer, and  $N$  the number of training samples.

This training process is repeated iteratively over multiple epochs until convergence. The network progressively adjusts its parameters to minimize the discrepancy between predicted and true outputs.

Although the concept of MLPs dates back several decades, the resurgence of deep learning has been driven by the availability of large datasets and advances in computing hardware. These developments have enabled the training of *deep* neural networks, which contain many layers and millions of parameters, dramatically increasing their representational power.

### 0.0.1 Convolutional Neural Networks

Convolutional Neural Networks (CNNs) are a class of deep learning models originally developed for image processing and now widely used across various domains. From LeCun’s early work on handwritten digit recognition in 1998<sup>S7</sup> to breakthroughs in large-scale image classification tasks such as ImageNet,<sup>S8</sup> CNNs have played a central role in advancing modern artificial intelligence.

CNNs extract hierarchical features from raw input data by convolving learnable filters (also called kernels) across the input space. Unlike traditional convolution operations with fixed filters, CNNs learn the filter weights during training via backpropagation, much like the weights in Multilayer Perceptrons (MLPs). This capacity to learn informative features directly from raw data makes CNNs particularly effective for modeling high-dimensional input signals.

A fundamental advantage of CNNs over fully connected networks is *weight sharing*. A single filter is applied repeatedly across different positions in the input, allowing the network to detect spatially recurring patterns while reducing the number of parameters. This property also confers *translational invariance*, meaning the network can recognize a feature regardless of its position in the input. These architectural advantages make CNNs well suited for tasks involving spatially structured inputs, such as images or sequential data.

A typical CNN architecture consists of three main types of layers: convolutional layers, pooling layers, and fully connected layers. Although real-world models use multiple filters, we will illustrate the core principles using a single-filter example.

**Convolutional Layers** Convolutional layers form the foundation of CNNs. Each layer applies a set of filters to the input by sliding them over the signal and computing element-wise multiplications followed by a summation. Figure S3 illustrates a 2D convolution example, where a  $3 \times 3$  kernel is applied to a single-channel input. The output at each location is computed as the dot product between the filter and the corresponding local region of the

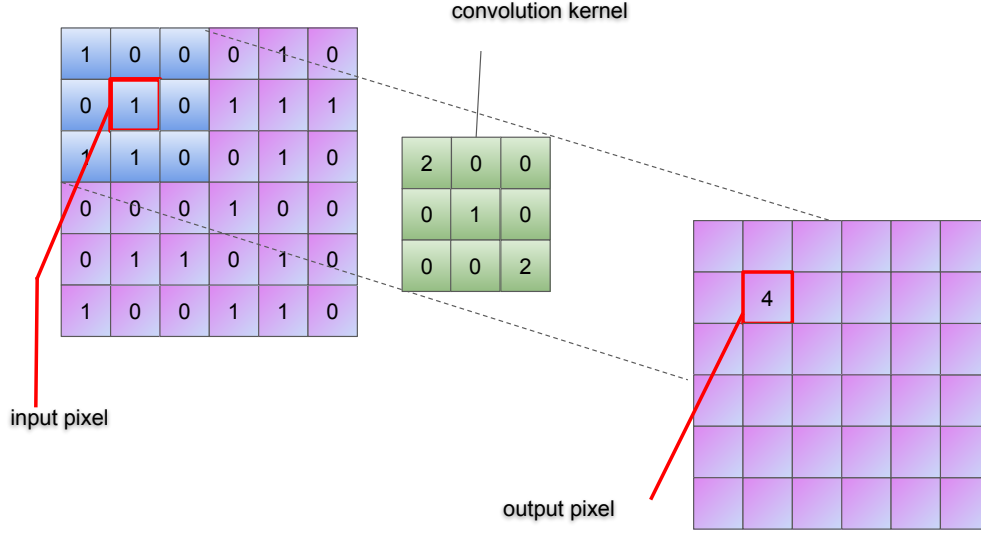

Figure S3: Example of a 2D convolution operation using a  $3 \times 3$  kernel on a single-channel image.

input.

For instance, consider a  $3 \times 3$  kernel with values arranged along the diagonal as  $\{2, 1, 2\}$ . If the input region matches the kernel pattern (e.g., values  $\{1, 1, 0\}$ ), the resulting output would be high, e.g.,  $1 \times 2 + 1 \times 1 + 0 \times 2 = 3$ . More formally, the 1D convolution operation can be written as:

$$S(t) = (x * w)(t) = \sum_n x(n)w(t - n), \quad (15)$$

where  $x(n)$  denotes the input signal and  $w(n)$  the convolution kernel. Convolution is a linear operation, so to model non-linear patterns, a non-linear activation function is applied to the output. Common activation functions include the Rectified Linear Unit (ReLU), sigmoid, and hyperbolic tangent.

**Relevance to Raman Spectroscopy** Although Raman spectra are one-dimensional signals, we include this explanation of 2D convolution to clarify CNN principles and highlight the challenges of applying CNNs to spectral data. In 2D image tasks, CNNs leverage in-

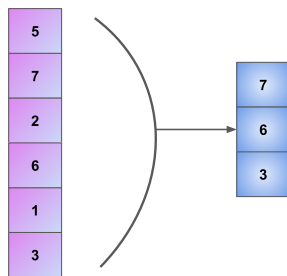

Figure S4: Illustration of a 1D max-pooling operation with a window size of 2.

ductive biases such as *local connectivity* and *spatial invariance*—both advantageous when features can appear anywhere in the image.

However, in Raman spectroscopy, this invariance is less desirable. Spectral peaks are localized and occur at specific Raman shifts that are critical for identifying molecular structures. If a CNN applies spatial invariance to Raman spectra, it may treat peaks at different positions as equivalent, potentially discarding vital information about molecular identity.

Therefore, adapting CNN architectures for Raman analysis requires careful modification of these biases. In particular, preserving the absolute positions of peaks is essential. Architectures for spectral data should use one-dimensional convolutions with reduced pooling to retain resolution along the spectral axis. These changes ensure that CNNs can effectively model the precise spectral patterns needed for accurate classification.

**Pooling Layers** Pooling layers reduce the spatial dimensionality of feature maps by summarizing local responses, thereby improving computational efficiency and helping mitigate overfitting. The most widely used pooling operation is *max pooling*, which retains the maximum value within a specified window of size  $m^2$ . This process preserves the most prominent features while discarding less significant variations. Figure S4 shows a one-dimensional (1D) max-pooling operation with  $m = 2$ .

---

<sup>2</sup>An alternative approach is average pooling, which computes the mean value within the same window.

While pooling is effective in image analysis—where features can appear in various positions and translation invariance is desirable—its application to Raman spectral data must be handled with care. In Raman spectroscopy, the absolute positions of spectral peaks along the Raman shift axis are essential for accurate molecular identification. Excessive pooling may blur or eliminate these peaks, leading to diminished sensitivity to fine spectral features and possible misclassification. Therefore, architectures designed for Raman data should use pooling layers judiciously, with window sizes selected to preserve the positional integrity of key spectral information.

**Fully Connected Layers** A typical CNN architecture consists of a sequence of convolutional and pooling layers, followed by one or more fully connected layers. In convolutional layers, each neuron is locally connected—that is, it receives input from only a small, spatially contiguous region of the preceding layer. For example, as shown in Figure S3, the highlighted output neuron is influenced by a  $3 \times 3$  region (nine neurons) from the previous feature map.

In contrast, fully connected layers establish connections between every neuron in one layer and all neurons in the preceding layer. This dense connectivity enables the network to integrate the local patterns extracted by the convolutional layers and to model complex, global relationships across the entire input. When paired with nonlinear activation functions, fully connected layers allow the model to learn intricate combinations of features, which is particularly useful for classification tasks.

Figure S5 illustrates a representative CNN architecture. The input image is shown in blue, followed by convolutional feature maps in yellow, a pooled feature map in orange, and fully connected layers in purple and green. These final layers synthesize the extracted features and map them to the output space, completing the decision-making process of the network.

**1D CNN for Raman Spectra** While the CNN architecture shown in Figure S5 is designed for two-dimensional (2D) inputs such as images, Raman spectra are fundamentally

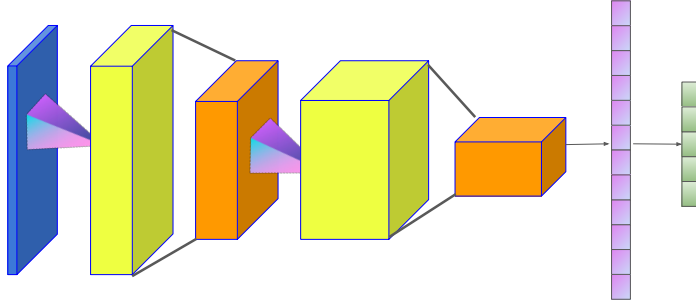

Figure S5: Illustrative example of a typical CNN architecture.

one-dimensional (1D) signals, with intensity values indexed by Raman shift. To process these spectral data effectively, we employ a one-dimensional convolutional architecture tailored to the structure of Raman signals.

Figure S6 illustrates a simplified example of a 1D convolution applied to a binary input vector, where a value of 1 indicates the presence of a peak and 0 indicates its absence. The convolution kernel in this example is defined as  $[-2, 4, -2]$ , designed to activate strongly when centered on a peak. The convolution at a given position  $t$  is computed as:

$$S(t) = \sum_n x(n) \cdot w(t - n), \quad (16)$$

where  $x(n)$  denotes the input signal,  $w(n)$  the kernel weights, and  $S(t)$  the output signal. For example, if the peak is centered at position  $t$ , the kernel response evaluates to  $S(t) = (-2 \times 0) + (4 \times 1) + (-2 \times 0) = 4$ .

Crucially, in a CNN, the kernel weights are not fixed but are learned during training via backpropagation. This allows the network to discover discriminative patterns in the data—such as peak positions, widths, and intensities—directly from raw spectra without requiring manual feature engineering.

While pooling layers can provide limited translation invariance, their use in spectral data must be approached with caution. In Raman spectroscopy, the absolute positions of spectral



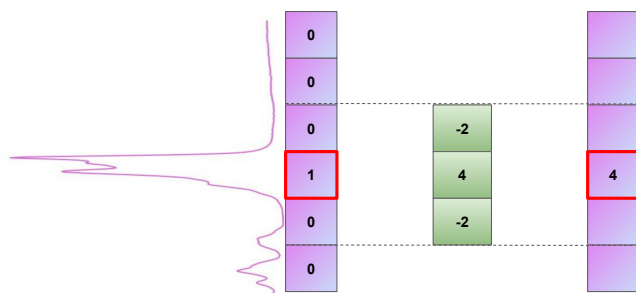

Figure S6: Illustration of a 1D convolution applied to a Raman spectrum using a kernel that responds selectively to peaks.

peaks carry significant chemical information. Excessive pooling may blur these features and degrade classification performance. To mitigate this, one can limit the depth or stride of pooling layers, or omit them entirely in favor of preserving high resolution along the spectral axis. This design choice allows the model to remain sensitive to meaningful spectral shifts while maintaining robustness against minor experimental noise.

## Semi-Supervised Learning

In many real-world scenarios, labeled data are scarce while unlabeled data are abundant. Semi-supervised learning provides a framework to exploit this imbalance by using unlabeled data to improve model performance when labels are limited. The central assumption is that the posterior class distribution  $p(\mathcal{C}|\mathbf{X})$  can be inferred more effectively when incorporating knowledge of the marginal input distribution  $p(\mathbf{X})$ .<sup>S9</sup> In other words, understanding the structure of the input space can help refine the classification boundary, even without direct access to labels.

Figure S7 shows a conceptual example of binary classification. The colored points represent labeled data, while the gray points represent unlabeled samples. In the absence of unlabeled data (left panel), the decision boundary is overly simplistic. Incorporating the unlabeled data (right panel) enables the model to learn a boundary that better reflects the

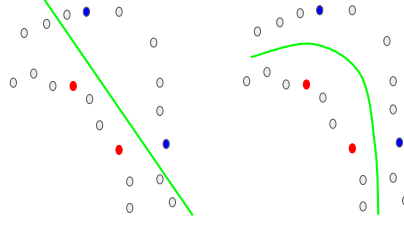

Figure S7: Illustrative example of semi-supervised learning. Left: decision boundary based only on labeled data. Right: boundary refined using unlabeled data.

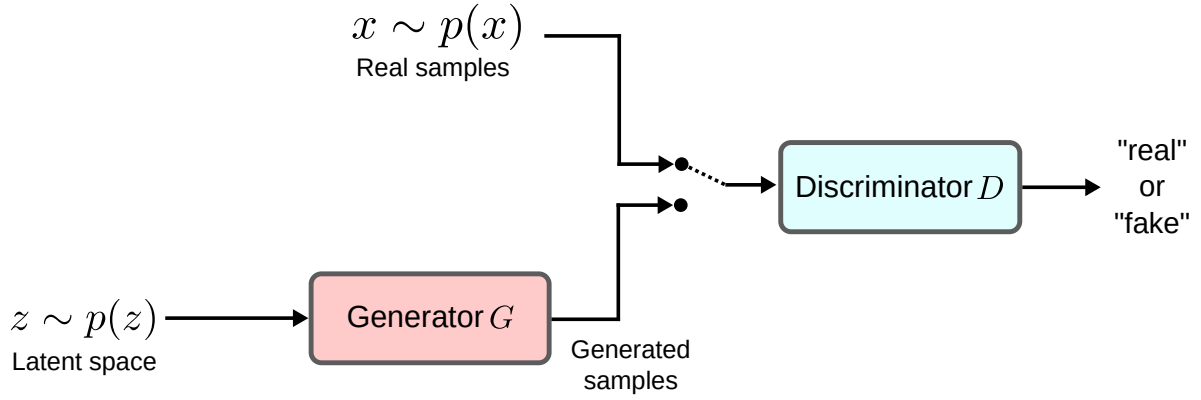

Figure S8: Architecture of a Generative Adversarial Network (GAN). Adapted from.<sup>S10</sup>

true data distribution. This refinement relies on the *smoothness assumption*, which posits that nearby points in the input space are likely to share the same label.

## 0.0.2 Semi-Supervised Generative Adversarial Networks

Generative Adversarial Networks (GANs) can be extended to semi-supervised learning, resulting in Semi-Supervised GANs (SGANs), which leverage both labeled and unlabeled data to improve classification performance.

**Generative Adversarial Networks** As illustrated in Figure S8, a standard GAN consists of two neural networks trained in opposition: a Generator ( $G$ ) and a Discriminator ( $D$ ). The Generator learns to map random noise vectors  $z \sim p_z(z)$  to synthetic samples that resemble real data drawn from a distribution  $p(\mathbf{X})$ . The Discriminator receives inputs that are either real data or generated data from the Generator, and outputs the probability that a sample

is real.

The objective of  $G$  is to generate data that  $D$  cannot distinguish from real samples, while  $D$  aims to correctly identify whether an input is real or generated. Formally, the GAN optimization problem is expressed as:<sup>S11</sup>

$$\begin{aligned} \min_G \max_D V(D, G) = & \mathbb{E}_{\mathbf{x} \sim p_{\text{data}}(\mathbf{x})} [\log D(\mathbf{x})] \\ & + \mathbb{E}_{\mathbf{z} \sim p_{\mathbf{z}}(\mathbf{z})} [\log(1 - D(G(\mathbf{z})))] \end{aligned} \quad (17)$$

where  $D(\mathbf{x})$  is the predicted probability that  $\mathbf{x}$  is a real sample, and  $G(\mathbf{z})$  is the output of the Generator. As training progresses,  $G$  learns to approximate the true data distribution  $p(\mathbf{X})$ , enabling the generation of realistic synthetic samples. GANs are widely used in applications such as image synthesis and data augmentation, where the trained Generator produces new data samples, and the Discriminator is typically used only during training.

**Semi-Supervised GANs** To incorporate unlabeled data, the SGAN framework modifies the role of the Discriminator. Instead of performing binary classification (real vs. fake),  $D$  is trained to classify inputs into  $K + 1$  categories: the original  $K$  real classes and an additional class representing synthetic data generated by  $G$ .<sup>S12</sup>

The Discriminator receives three types of input: labeled real samples, unlabeled real samples, and generated (synthetic) samples. Its objectives are as follows:

1. Classify labeled real samples correctly into one of the  $K$  real classes.
2. Assign unlabeled real samples to one of the  $K$  real classes, acknowledging their authenticity.
3. Assign generated samples to the  $(K + 1)^{\text{th}}$  class, identifying them as synthetic.

This design enables  $D$  to simultaneously act as a classifier and a detector of synthetic data, using adversarial training to improve generalization.

The SGAN objective function combines a supervised loss term with an unsupervised adversarial loss:

$$\begin{aligned}
L &= L_{\text{supervised}} + L_{\text{unsupervised}}, \\
L_{\text{supervised}} &= -\mathbb{E}_{(\mathbf{x}, y) \sim p_{\text{data}}} \log p_{\text{model}}(y \mid \mathbf{x}, y \leq K), \\
L_{\text{unsupervised}} &= -\mathbb{E}_{\mathbf{x} \sim p_{\text{data}}} \log[1 - p_{\text{model}}(y = K + 1 \mid \mathbf{x})] \\
&\quad - \mathbb{E}_{\mathbf{x} \sim G} \log[p_{\text{model}}(y = K + 1 \mid \mathbf{x})],
\end{aligned} \tag{18}$$

Here,  $L_{\text{supervised}}$  encourages accurate classification of labeled data, while  $L_{\text{unsupervised}}$  penalizes the Discriminator for misclassifying real samples as synthetic and rewards it for correctly identifying synthetic samples. This formulation enables the model to benefit from unlabeled data and adversarial feedback, enhancing its capacity to generalize from limited supervision.

### 0.0.3 Contrastive Learning

In the context of unsupervised representation learning for Raman spectra, contrastive learning has emerged as a promising approach. Although initially introduced to improve few-shot learning in supervised settings, contrastive methods have since gained popularity in self-supervised learning frameworks, where label information is unavailable.<sup>S13</sup>

In this work, we adopt the SimCLR framework introduced by Chen *et al.*,<sup>S14</sup> which learns useful representations by maximizing agreement between different augmented views of the same sample. Specifically, two stochastic augmentations,  $T(\cdot)$  and  $T'(\cdot)$ , are independently applied to each input sample, producing a positive pair. These augmented inputs are passed through an encoder network  $f(\cdot)$  to extract high-level features, followed by a projection head  $g(\cdot)$  that maps the encoded representations into a latent space. The similarity between representations is measured using cosine similarity:

$$\text{sim}(\mathbf{z}, \mathbf{z}') = \frac{\mathbf{z}^\top \mathbf{z}'}{\|\mathbf{z}\| \cdot \|\mathbf{z}'\|}, \quad (19)$$

where  $\mathbf{z}$  and  $\mathbf{z}'$  are the projected representations of the augmented inputs, and  $\|\cdot\|$  denotes the Euclidean norm.

To train the network, a contrastive loss is applied that encourages the representations of positive pairs to be similar, while pushing apart those of negative pairs. For a positive pair  $(i, j)$  within a batch of  $2N$  augmented examples, the contrastive loss is defined as:

$$L_{i,j} = -\log \frac{\exp(\text{sim}(\mathbf{z}_i, \mathbf{z}_j)/\tau)}{\sum_{k=1}^{2N} \mathbb{1}_{[k \neq i]} \exp(\text{sim}(\mathbf{z}_i, \mathbf{z}_k)/\tau)}, \quad (20)$$

where  $\tau$  is a temperature parameter that controls the concentration of the distribution, and  $\mathbb{1}_{[k \neq i]}$  is an indicator function equal to 1 when  $k \neq i$  and 0 otherwise. Each positive pair is formed by two augmentations of the same original input, while the remaining  $2(N - 1)$  examples in the batch serve as negative samples.

For Raman spectroscopy, the effectiveness of contrastive learning strongly depends on appropriate data augmentations that preserve the underlying chemical identity of the sample. Useful augmentation strategies include:

- **Additive noise:** Mimicking measurement noise to increase robustness.
- **Intensity scaling:** Varying signal amplitude to reflect experimental variability.
- **Peak shifting:** Slightly translating spectral peaks to simulate calibration errors while maintaining chemical interpretability.

By leveraging these transformations, contrastive learning enables the model to discover latent structure in the spectral data without requiring labels, laying the groundwork for downstream tasks such as classification or clustering.

## Training and Validation Loss Curves

To assess convergence and over-/under-fitting, we plot the training and validation loss curves for our MLP variants and the 1-D CNN on both RRUFF-raw and RRUFF-clean datasets.

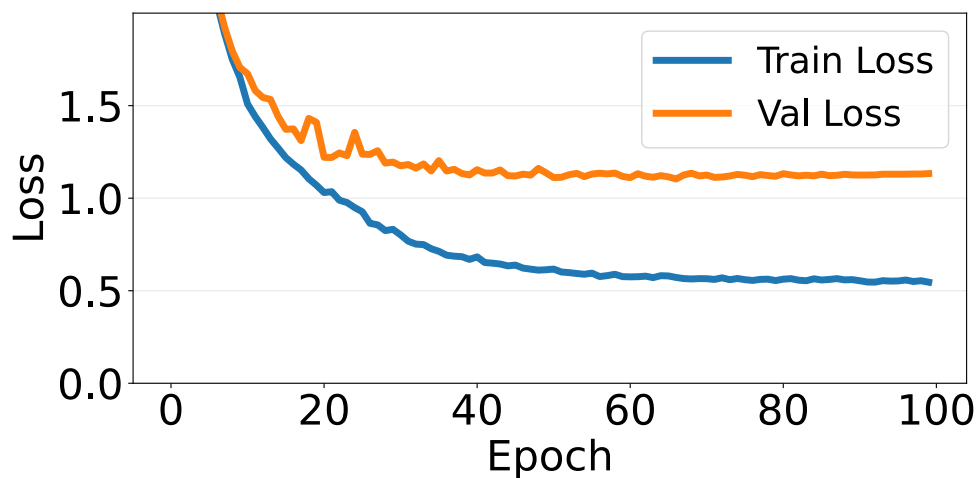

Figure S9: Training and validation categorical cross-entropy loss for **MLP-small** on the **RRUFF-raw** dataset. Persistent high validation loss indicates underfitting.

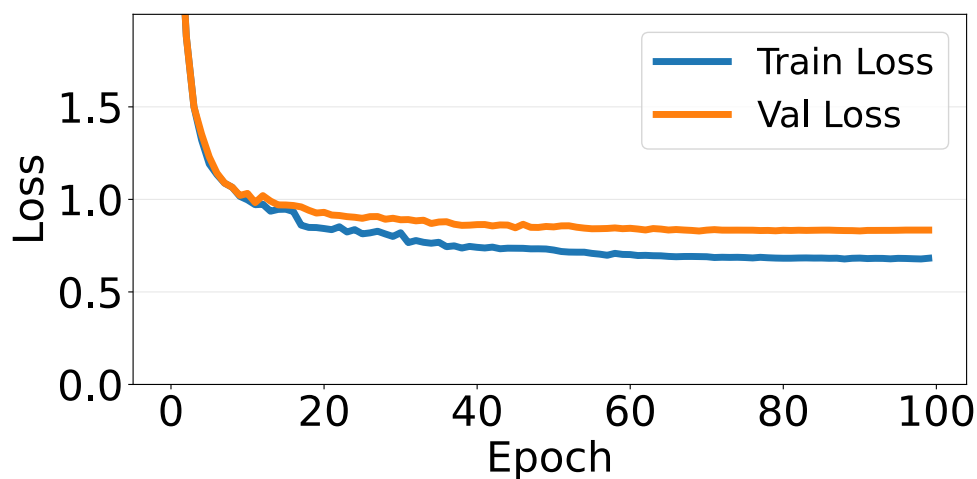

Figure S10: Training and validation categorical cross-entropy loss for **MLP-small** on the **RRUFF-clean** dataset.

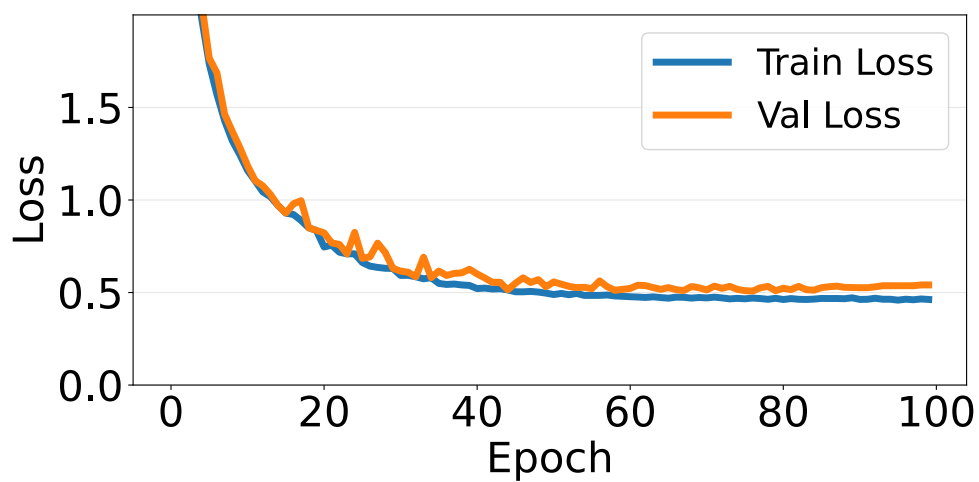

Figure S11: Training and validation categorical cross-entropy loss for **MLP-mid** on the **RRUFF-raw** dataset.

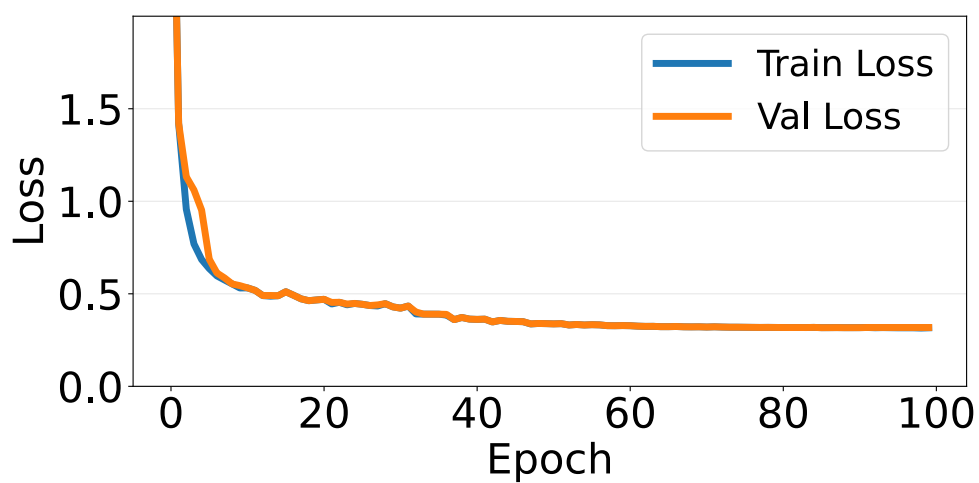

Figure S12: Training and validation categorical cross-entropy loss for **MLP-mid** on the **RRUFF-clean** dataset.

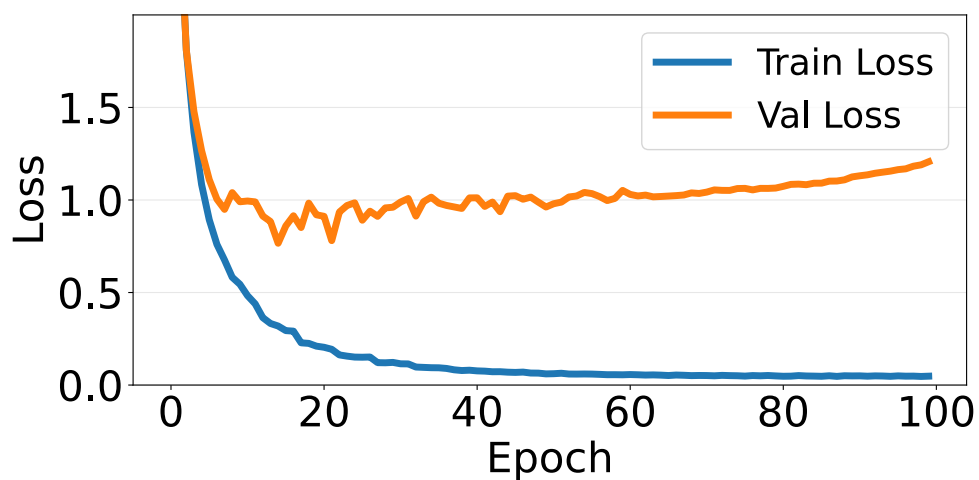

Figure S13: Training and validation categorical cross-entropy loss for **MLP-large** on the **RRUFF-raw** dataset. A widening gap indicates overfitting.

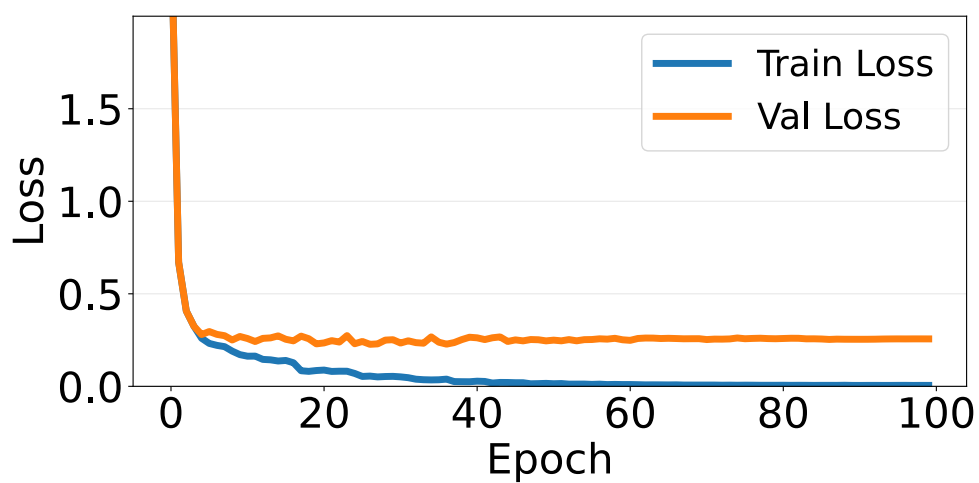

Figure S14: Training and validation categorical cross-entropy loss for **MLP-large** on the **RRUFF-clean** dataset.



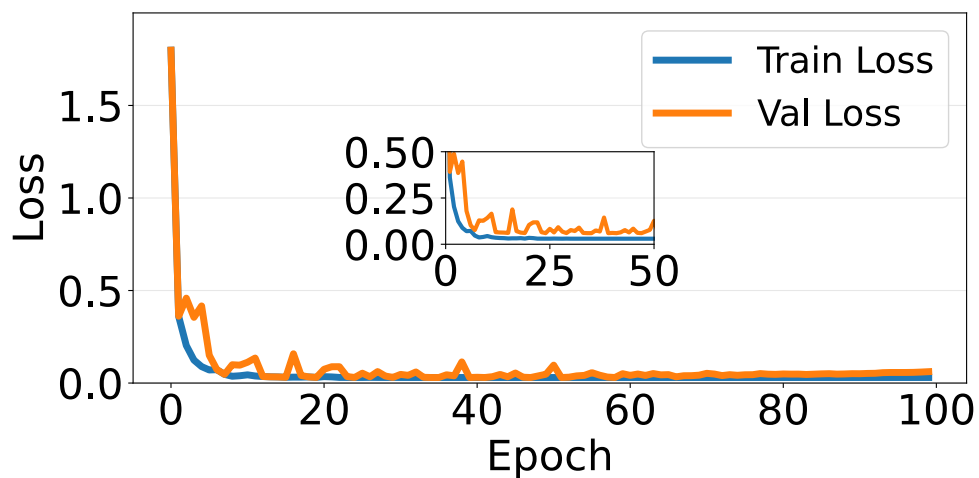

Figure S15: Training and validation categorical cross-entropy loss for **CNNs** on the **RRUFF-raw** dataset. Fast convergence and small generalization gap highlight strong fit.

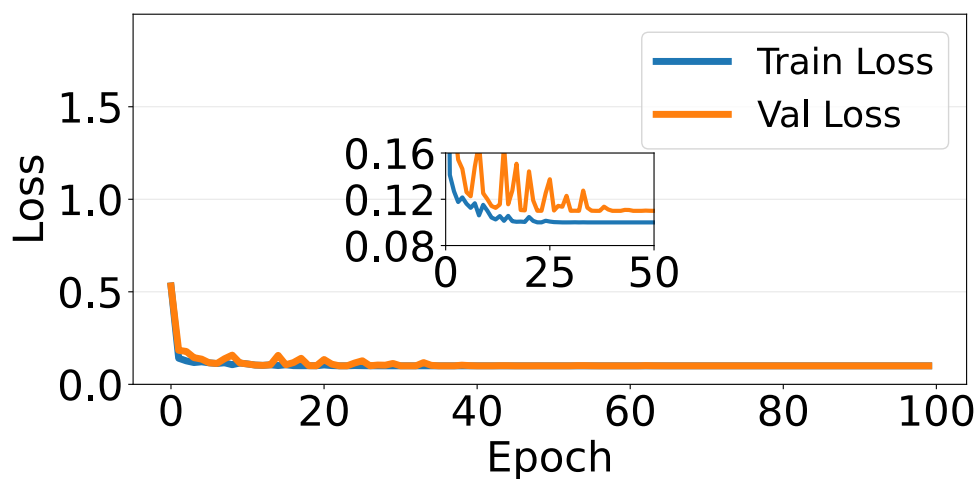

Figure S16: Training and validation categorical cross-entropy loss for **CNNs** on the **RRUFF-clean** dataset.

# Transfer Learning Fine-Tuning Curves

Here we add the training curves for the transfer learning experiments.

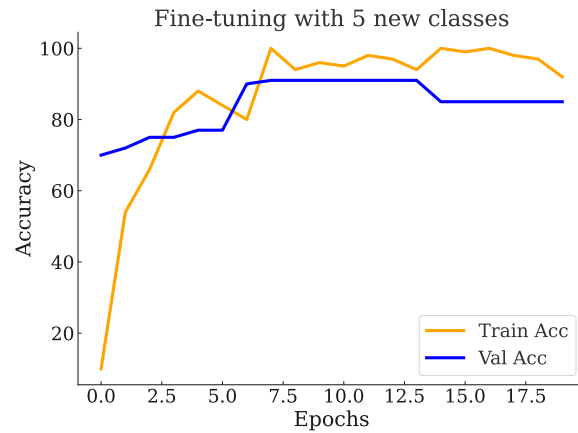

Figure S17: Fine-tuning training and validation Top-1 accuracy for  $c = 5$  new classes.

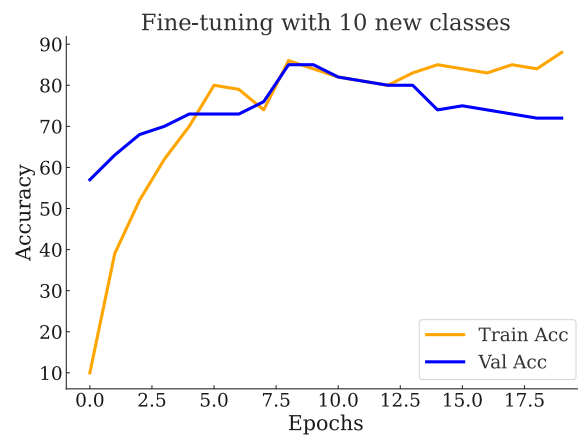

Figure S18: Fine-tuning training and validation Top-1 accuracy for  $c = 10$  new classes.

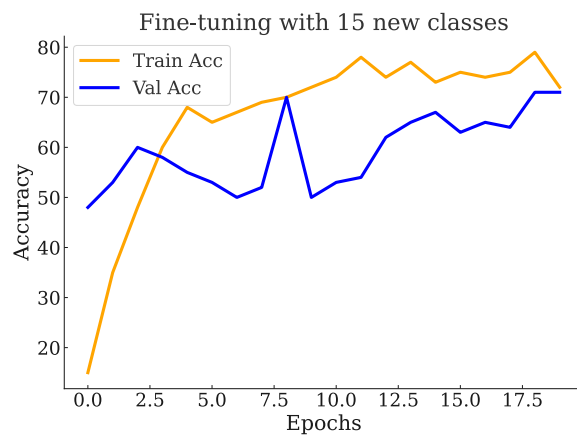

Figure S19: Fine-tuning training and validation Top-1 accuracy for  $c = 15$  new classes.

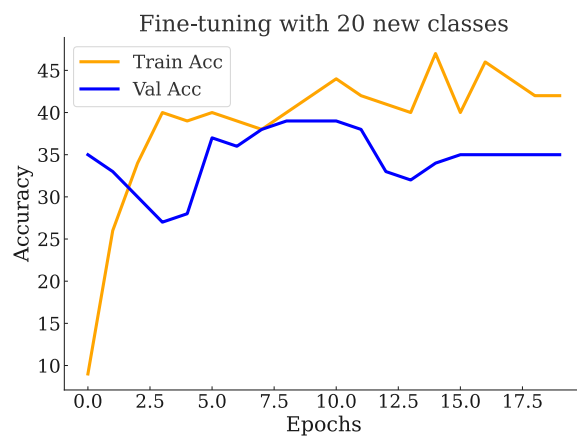

Figure S20: Fine-tuning training and validation Top-1 accuracy for  $c = 20$  new classes.

## References

- (S1) Ball, G. H.; Hall, D. J. *ISODATA, a Novel Method of Data Analysis and Pattern Classification*; 1965.
- (S2) Pearson, K. On Lines and Planes of Closest Fit to Systems of Points in Space. *Lond. Edinb. Dubl. Philos. Mag. J. Sci.* **1901**, *2*, 559–572.
- (S3) Hotelling, H. Analysis of a Complex of Statistical Variables into Principal Components. *J. Educ. Psychol.* **1933**, *24*, 417–441.
- (S4) Jebara, T. *Machine Learning: Discriminative and Generative*; Springer Science & Business Media, 2012; Vol. 755.
- (S5) Vapnik, V. N. *The Nature of Statistical Learning Theory*; Springer-Verlag, 1995.
- (S6) Cover, T.; Hart, P. Nearest Neighbor Pattern Classification. *IEEE Trans. Inf. Theory* **1967**, *13*, 21–27.
- (S7) LeCun, Y.; Bottou, L.; Bengio, Y.; Haffner, P. Gradient-Based Learning Applied to Document Recognition. *Proc. IEEE* **1998**, *86*, 2278–2324.
- (S8) Alom, M. Z.; Taha, T.; Yakopcic, C.; Westberg, S.; Sidike, P.; Nasrin, M.; Hasan, M.; Essen, B.; Awwal, A.; Asari, V. A State-of-the-Art Survey on Deep Learning Theory and Architectures. *Electronics* **2019**, *8*, 292.
- (S9) van Engelen, J. E.; Hoos, H. H. A Survey on Semi-Supervised Learning. *Mach. Learn.* **2020**, *109*, 373–440.
- (S10) Ouali, Y.; Hudelot, C.; Tami, M. An Overview of Deep Semi-Supervised Learning. 2020; arXiv preprint arXiv:2006.05278.

- (S11) Goodfellow, I.; Pouget-Abadie, J.; Mirza, M.; Xu, B.; Warde-Farley, D.; Ozair, S.; Courville, A.; Bengio, Y. Generative Adversarial Nets. *Adv. Neural Inf. Process. Syst.* 2014.
- (S12) Salimans, T.; Goodfellow, I.; Zaremba, W.; Cheung, V.; Radford, A.; Chen, X. Improved Techniques for Training GANs. *Adv. Neural Inf. Process. Syst.* 2016.
- (S13) Tian, Y.; Sun, C.; Poole, B.; Krishnan, D.; Schmid, C.; Isola, P. What Makes for Good Views for Contrastive Learning. *CoRR* **2020**, *abs/2005.10243*.
- (S14) Chen, T.; Kornblith, S.; Norouzi, M.; Hinton, G. A Simple Framework for Contrastive Learning of Visual Representations. *Proc. Int. Conf. Mach. Learn.* 2020; pp 1597–1607.
